# Supplementary material for: Automating reward function configuration for drug design
Source: arXiv:2312.09865 source file (2023-12-15)
Supplement: Supplementary file 1 [file supplemental.tex]

\section{Supplementary Material}
